# Supplementary material for: Learning Image-Adaptive Codebooks for Class-Agnostic Image Restoration
Source: arXiv:2306.06513 source file (2023-06-13)
Supplement: Supplementary file 2 [file supplement.pdf]

# Learning Image-Adaptive Codebooks for Class-Agnostic Image Restoration (Supplementary material)

## A. Semantic Grouped Classes

As described in the paper, we aggregate the 150 classes in ADE20K dataset [4] into five super-classes to train our basis codebooks. The overall details of how we divide the five sub-datasets are shown in Fig. 1. Although this is not a rigorous categorization, the codebook visualization in Section 3.1 empirically demonstrates that the grouping is meaningful to some extent.

## B. Network Architectures

In conjunction with the encoder-decoder network used in our AdaCode, we elaborate on the detailed architectures of the encoder  $E$ , the decoder  $G$ , and the discriminator  $D$ . For  $E$  and  $G$ , we adopt the same autoencoder as VQGAN [2] in stage I and the same structure as FeMaSR [1] in stage II&III. For  $D$ , we adopt the same U-Net discriminator with spectral normalization as Real-ESRGAN [3].

## C. More Results

### C.1. Ablation on Codebook Size

We conduct experiments to empirically select the number of code entries in each basis codebook, as shown in Table. 1. Considering the tradeoff between performance and computation cost, we set the basis codebooks' size as  $\{512, 256, 512, 256, 256\} \times 256$ .

### C.2. Codebook Visualization

We visualize all the codes in our five basis codebooks in Fig. 2. As we discussed in Section 5, it is yet unclear how many basis codebooks and how many code entries in each codebook we need. It is also reflected by the visualization that there might be some redundancies in the codebooks.

### C.3. Qualitative Results

We show more results and comparisons for image reconstruction, super-resolution, and image inpainting in Fig. 3, Fig. 4, and Fig. 5, which empirically demonstrate the effectiveness of AdaCode.

Table 1: Stage I reconstruction performance on each super-class with different number of code entries. The chosen size is marked in red.

| Super-Class    | Codebook Size    | PSNR   | SSIM  | LPIPS |
|----------------|------------------|--------|-------|-------|
| Architectures  | $256 \times 256$ | 24.096 | 0.667 | 0.149 |
|                | $512 \times 256$ | 24.260 | 0.684 | 0.144 |
| Indoor Objects | $256 \times 256$ | 26.565 | 0.788 | 0.110 |
|                | $512 \times 256$ | 26.630 | 0.789 | 0.110 |
| Natural Scenes | $256 \times 256$ | 27.014 | 0.723 | 0.124 |
|                | $512 \times 256$ | 27.693 | 0.743 | 0.110 |
| Street Views   | $256 \times 256$ | 26.677 | 0.748 | 0.126 |
|                | $512 \times 256$ | 26.937 | 0.755 | 0.127 |
| Portraits      | $256 \times 256$ | 29.914 | 0.838 | 0.097 |
|                | $512 \times 256$ | 29.662 | 0.837 | 0.098 |

## References

- [1] Chaofeng Chen, Xinyu Shi, Yipeng Qin, Xiaoming Li, Xiaoguang Han, Tao Yang, and Shihui Guo. Real-World Blind Super-Resolution via Feature Matching with Implicit High-Resolution Priors. In *Proceedings of ACM International Conference on Multimedia (MM)*, 2022.
- [2] Patrick Esser, Robin Rombach, and Bjorn Ommer. Taming Transformers for High-Resolution Image Synthesis. In *Proceedings of the IEEE/CVF Conference on Computer Vision and Pattern Recognition (CVPR)*, 2021.
- [3] Xintao Wang, Liangbin Xie, Chao Dong, and Ying Shan. Real-ESRGAN: Training Real-World Blind Super-Resolution With Pure Synthetic Data. In *Proceedings of the IEEE/CVF International Conference on Computer Vision (ICCV)*, 2021.
- [4] Bolei Zhou, Hang Zhao, Xavier Puig, Sanja Fidler, Adela Barriuso, and Antonio Torralba. Scene Parsing through ADE20K Dataset. In *Proceedings of the IEEE conference on computer vision and pattern recognition (CVPR)*, 2017.

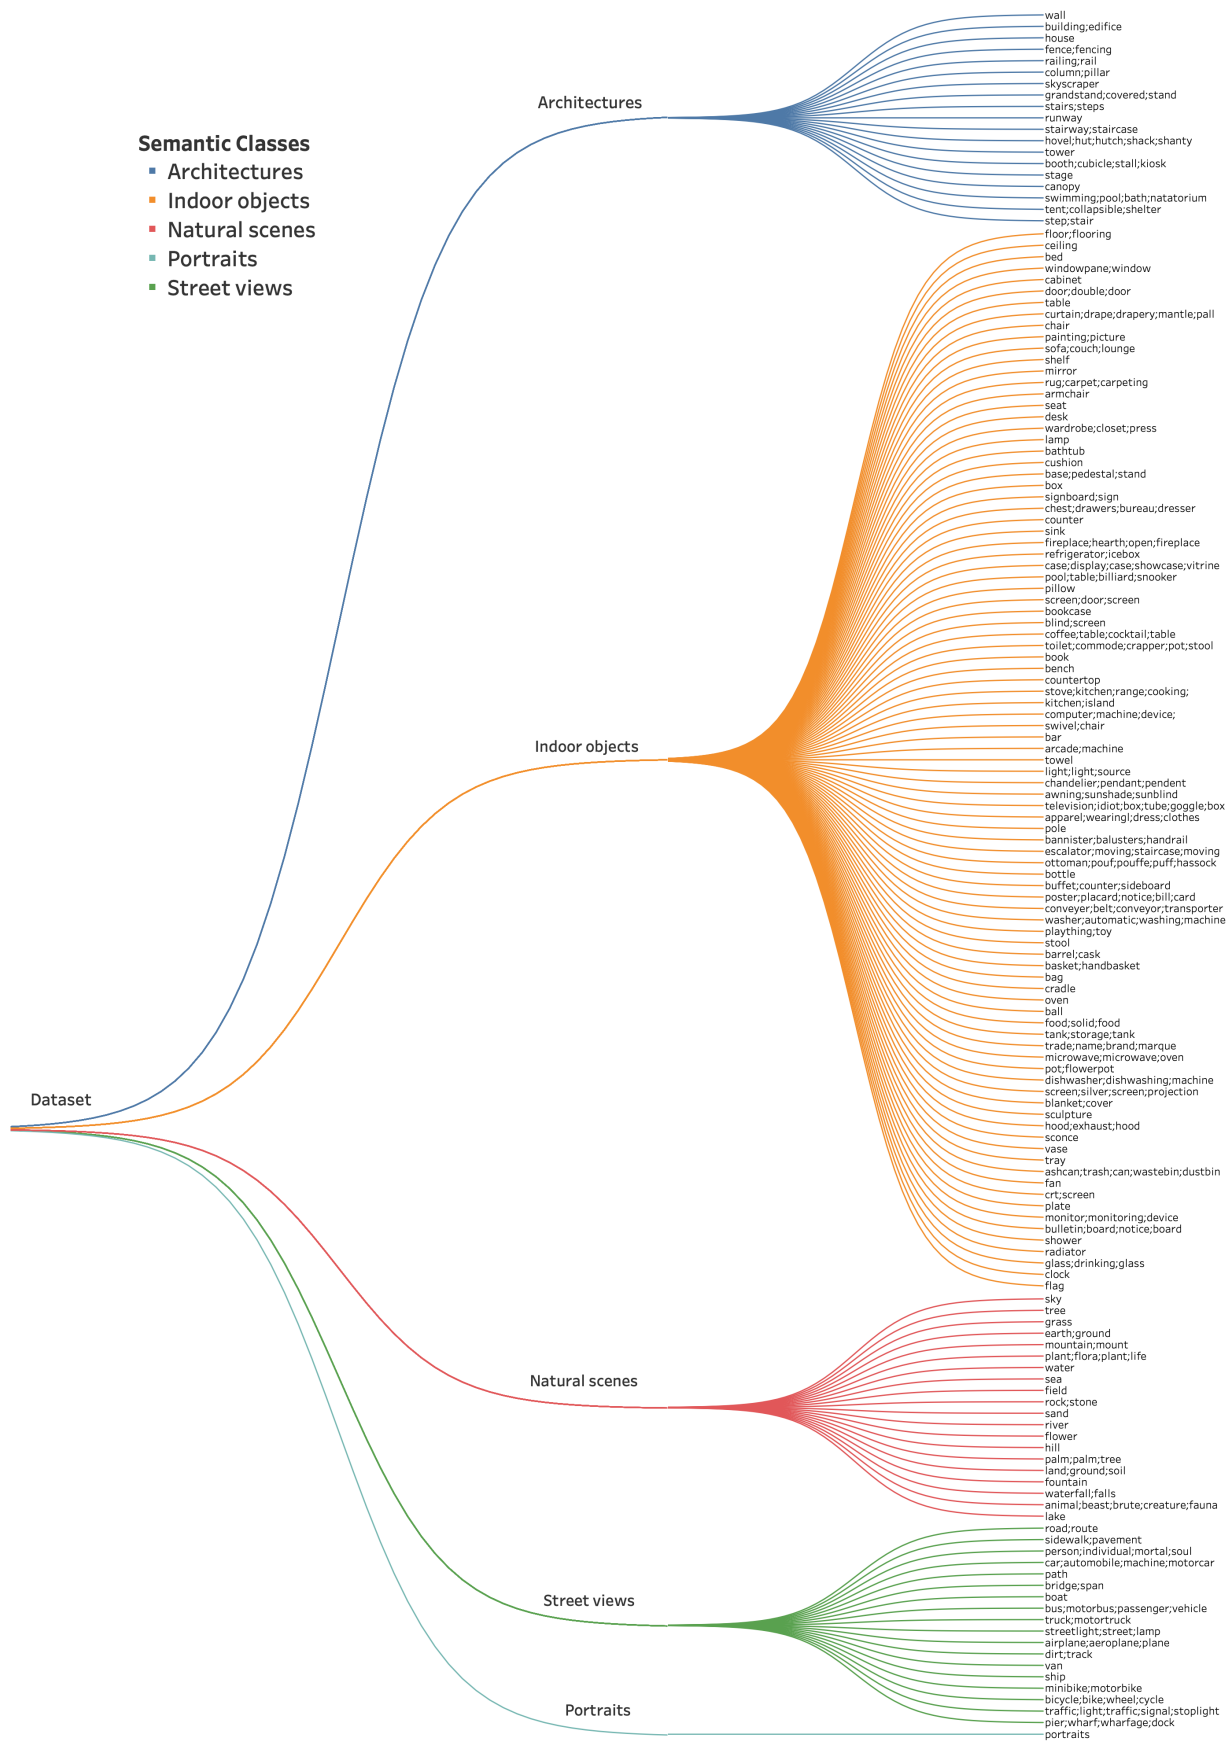

Figure 1: Groups of 150 classes in ADE20K dataset [4].

$Z_1$ : Architecture

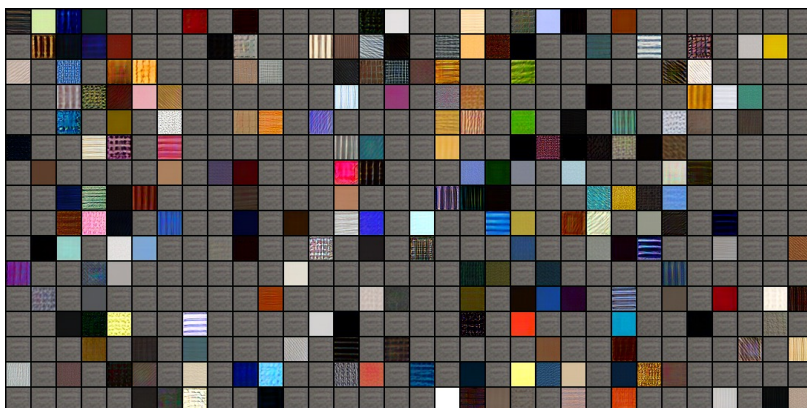

$Z_2$ : Indoor Objects

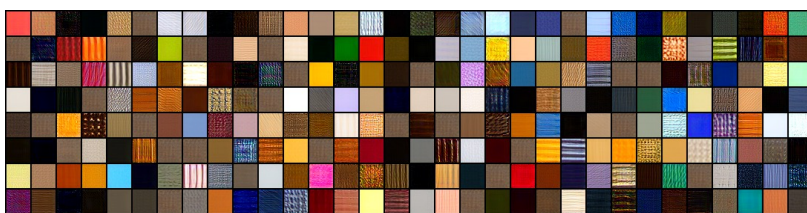

$Z_3$ : Natural Scenes

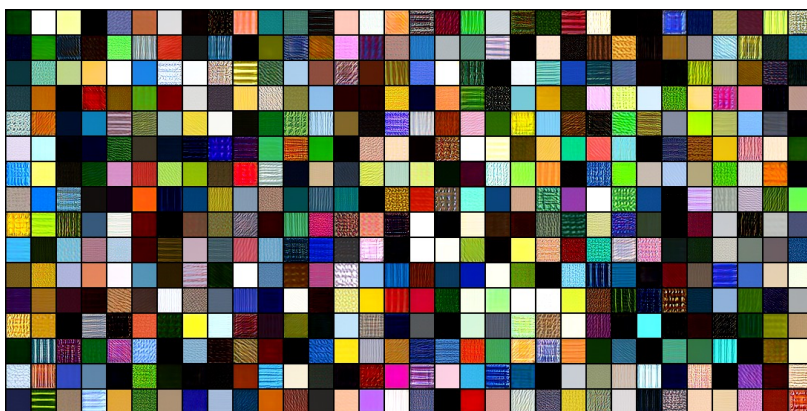

$Z_4$ : Street Views

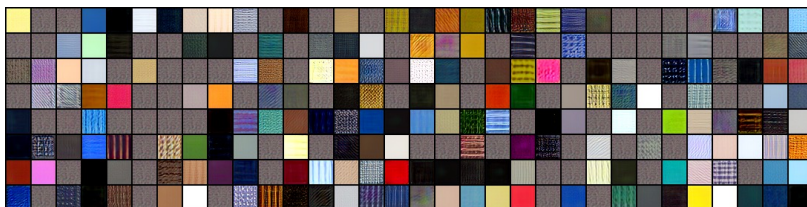

$Z_5$ : Portraits

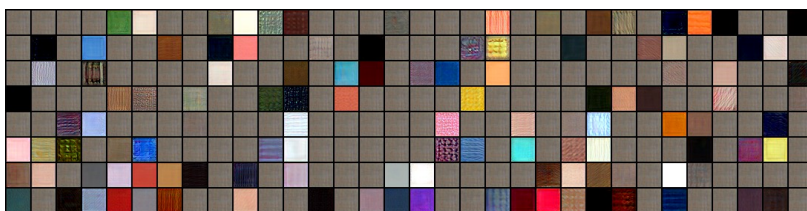

Figure 2: Visualization of all the basis codebooks.



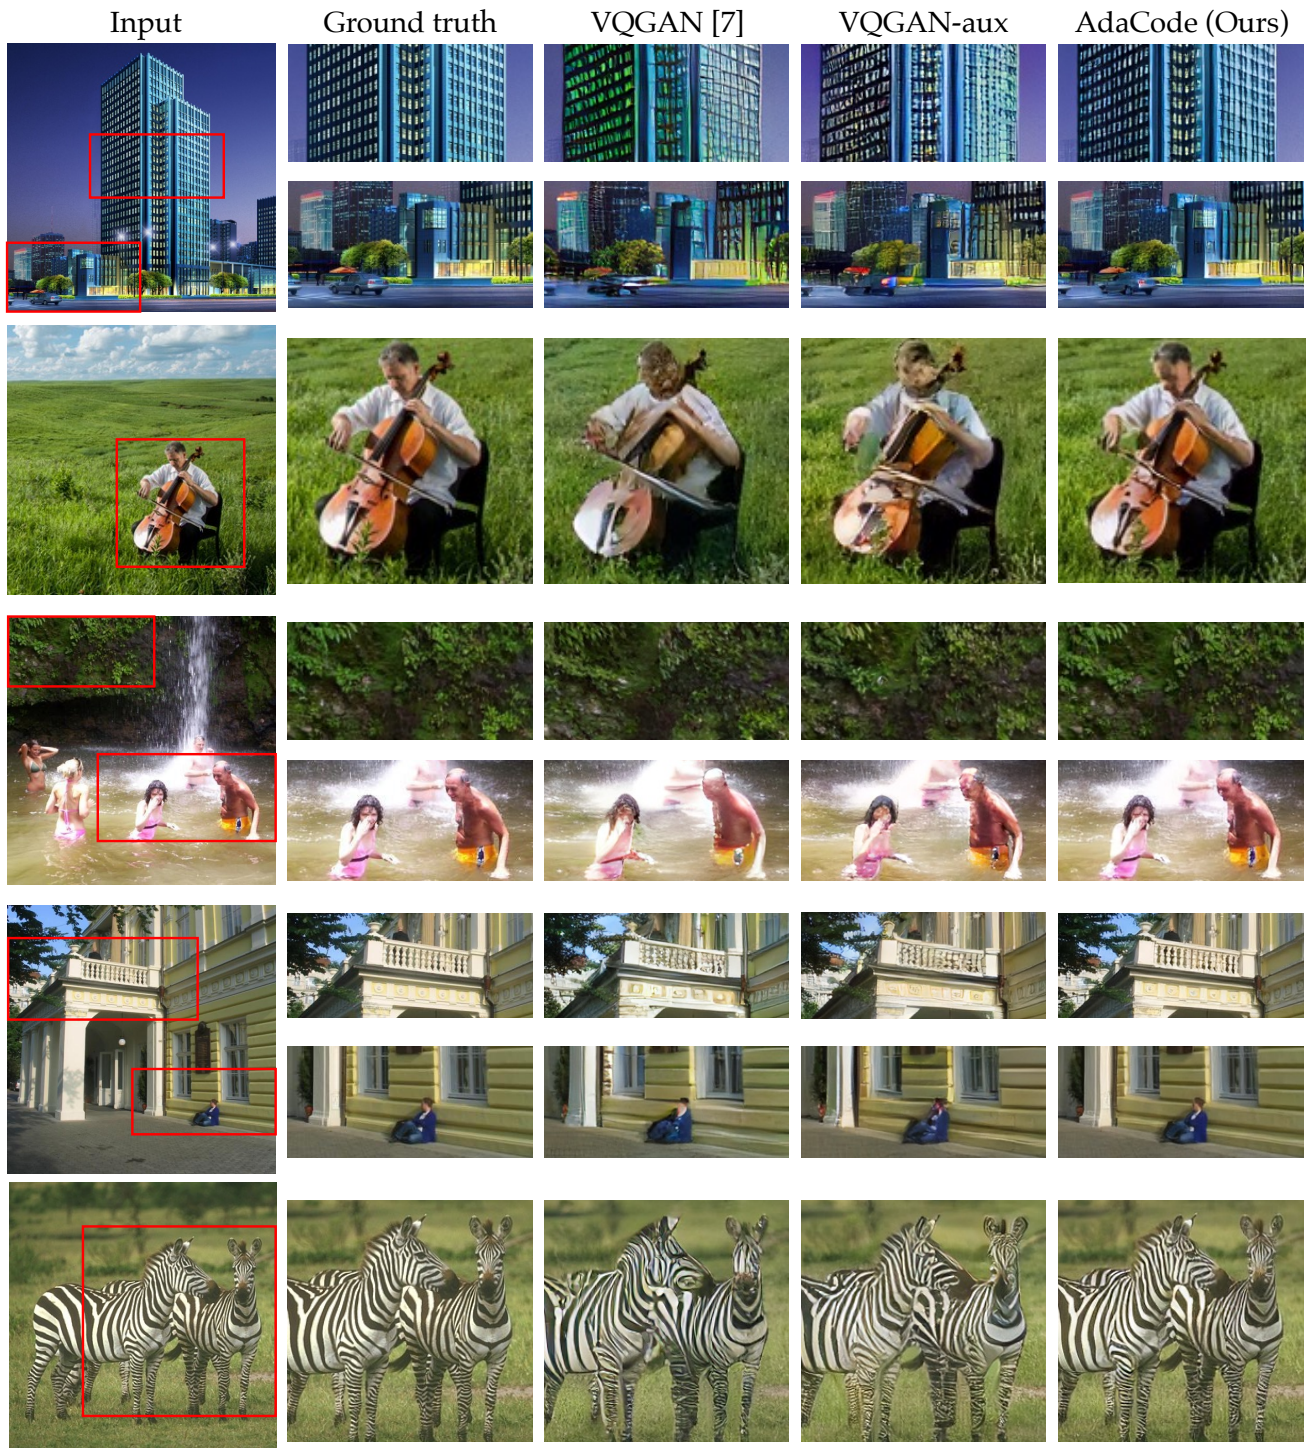

Figure 3: More results on Image Reconstruction.



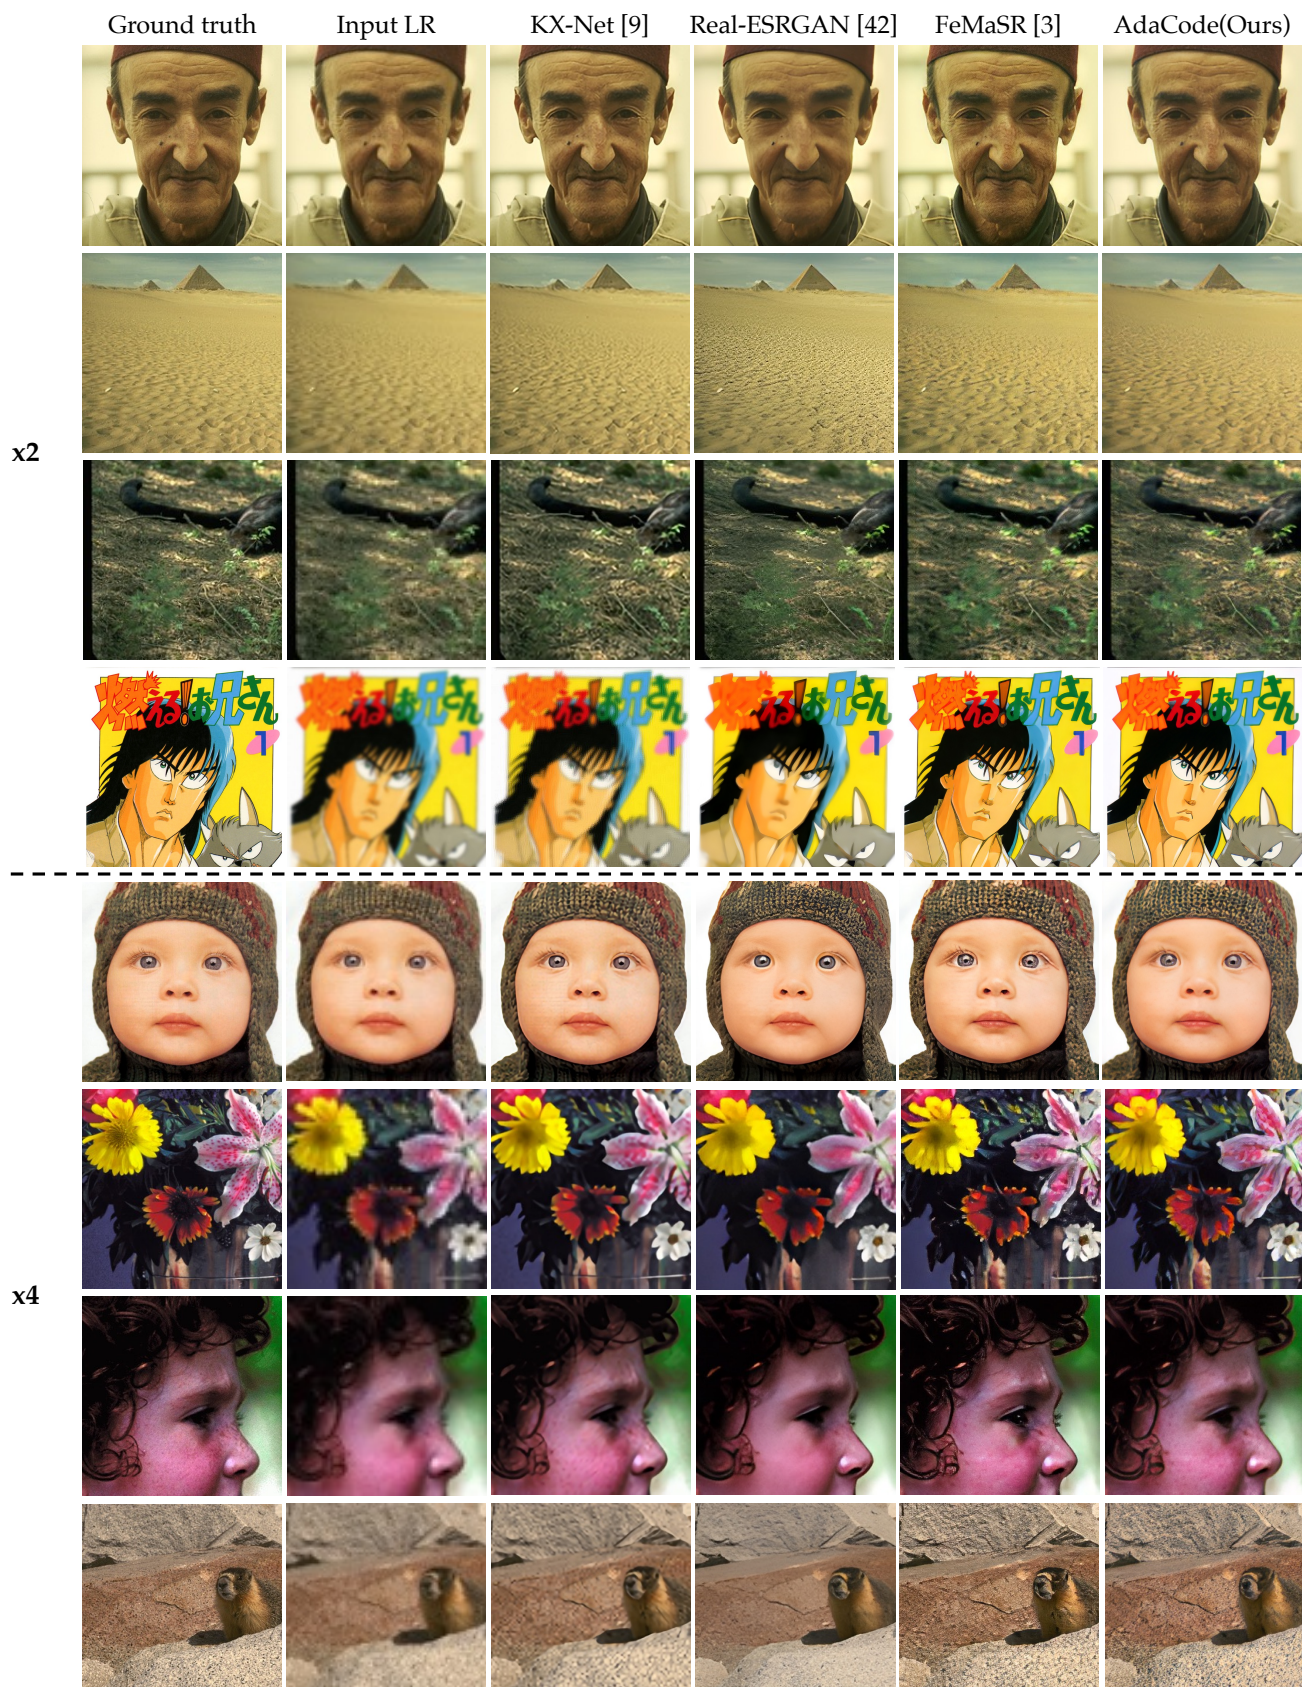

Figure 4: More results on Super-Resolution.



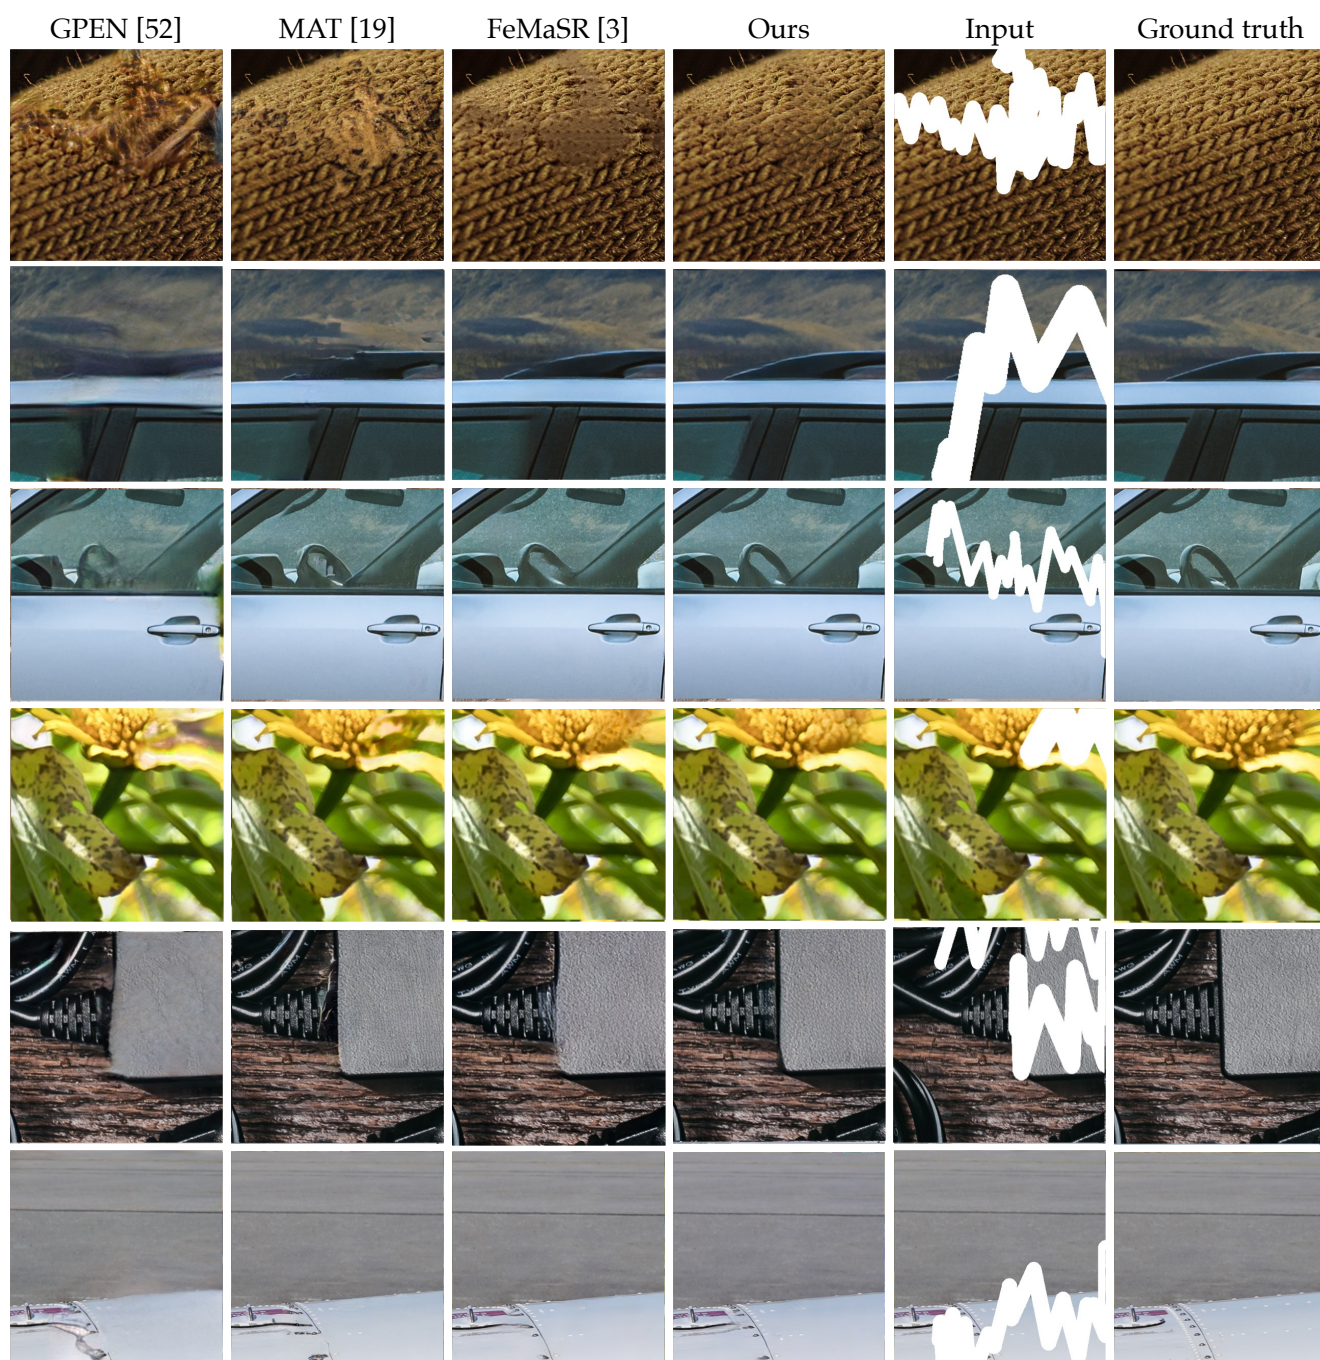

Figure 5: **More results on Image Inpainting.**
